# Supplementary material for: Magnetoresistance from broken spin helicity
Source: arXiv:1412.4065 source file (2014-12-12)
Supplement: Supplementary file 1 [file supplementary_information.pdf]

# Magnetoresistance from broken spin helicity: Supplementary Information

D.P. Leusink,[1] R.G.J. Smits,[1] P. Ngabonziza,[1] X.L. Wang,[2] S. Wiedmann,[3] U. Zeitler,[3] and A. Brinkman[1]

[1]*Faculty of Science and Technology and MESA+ Institute for Nanotechnology, University of Twente, The Netherlands*

[2]*Institute for Superconducting and Electronic Materials, University of Wollongong, Wollongong, Australia*

[3]*High Field Magnet Laboratory, Institute of Molecules and Materials, Radboud University Nijmegen, The Netherlands*

(Dated: December 12, 2014)

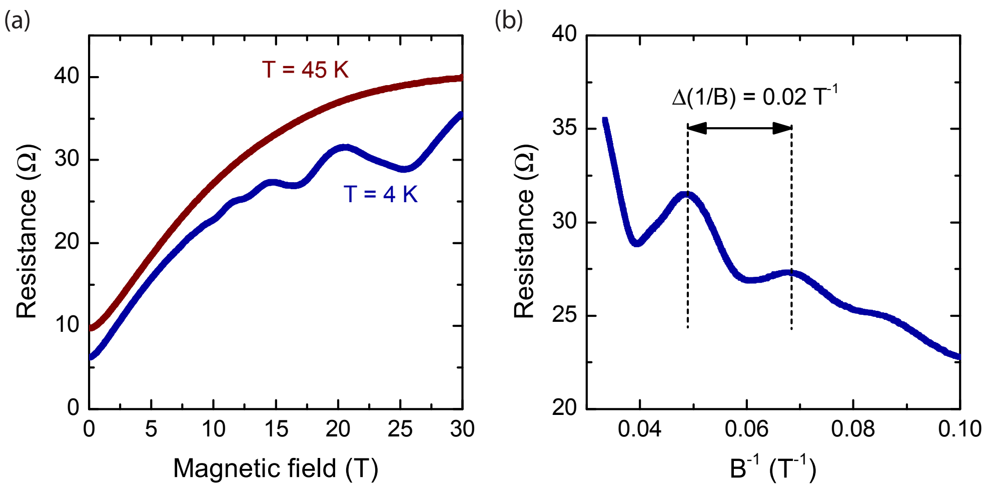


FIG. 1: **Figure S1 — Shubnikov-de Haas oscillations in $Bi_2Te_3$** (a) Magnetoresistance of the $Bi_2Te_3$ Hall bar at 45 K and 4 K. (b) The 4 K magnetoresistance shows Shubnikov-de Haas oscillations that are periodic in $\frac{1}{B}$.

### 1. Contribution of the topological surface states

Figure S1 shows the magnetoresistance of the $Bi_2Te_3$ Hall bar at different temperatures. At 4 K, clear Shubnikov-de Haas oscillations can be seen, with a periodicity of $\Delta\left(\frac{1}{B}\right) = 0.02\ \mathrm{T}^{-1}$. This periodicity corresponds to a carrier density of $1.2 \times 10^{12}\ \mathrm{cm}^{-2}$, consistent with previous samples from similar crystals [1]. The value is also perfectly consistent ($n = \frac{k_F^2}{4\pi}$) with the value for the Fermi wavevector of $k_F = 0.04\ \text{Å}^{-1}$ that was obtained in the main text for the parabolic conduction band, assuming that the topological surface state Dirac cone dispersion is very close to the parabolic bulk band dispersion. The disappearance of the oscillations at 45 K puts an upper bound to the mobility of the carriers of the topological surface state. This allows us to ignore the topological surface state contribution to the longitudinal and transverse conductance at 45 K. At lower temperatures, the contribution from the topological surface state increases, as seen from the amplitude of the quantum oscillations, and also an increase of the overall conduction can be seen, which can both be attributed to the topological surface states or additional trivial surface states (such as calculated for $Bi_2Se_3$ [2]). For the analysis of the main text, trivial two-dimensional electron gases and bulk states are both characterized by spin-split parabolic bands and can be treated on an equal footing.

### 2. Beyond the one-band model

For Zeeman and/or spin-orbit energies that are not much smaller than the Fermi energy, the band splitting at the Fermi is relatively large and two-band equations should be used for the conductivity. Within the helical magnetoresistance model the standard two-band equations for conductivity should be supplemented by magnetic field dependent carrier densities, i.e.

$$\sigma_{xx} = \sigma_{xx}^{+} + \sigma_{xx}^{-} = \frac{en_{+}(B)\mu_{+}(B)}{1+[\mu_{+}(B)B]^2} + \frac{en_{-}(B)\mu_{-}(B)}{1+[\mu_{-}(B)B]^2}, \tag{1}$$

$$\sigma_{xy} = \sigma_{xy}^{+} + \sigma_{xy}^{-} = B\mu_{+}(B)\sigma_{xx}^{+} + B\mu_{-}(B)\sigma_{xx}^{-}, \tag{2}$$

where $\mu_{\pm}(B)$ follows the helical magnetoresistance model, such as given by the inverse of Eq. (2) in the main text. Under constant Fermi energy condition, the spectral weight transfer from $n_{+}$ to $n_{-}$ as function of increasing values of $B$ can be calculated directly from the $k_{F\pm}$ that can be obtained from the complete dispersion relation. When the Zeeman energy becomes so large that $n_{+}$ gets completely depleted (when its entire dispersion relation falls above $E_F$), one cannot any longer sustain the condition of a constant Fermi energy. Rather, $n_{-}$ becomes constant and $E_F$ adapts to that condition. If, for some extrinsic reason (such as the presence of an additional impurity band), the Fermi energy is pinned, then also $n_{-}$ can become magnetic field dependent after depletion of $n_{+}$.

### 3. Helical magnetoresistance model for arbitrary field direction

The Hamiltonian for our helical magnetoresistance model is given by

$$H = \frac{\hbar^2 k^2}{2m_0} + \frac{\alpha}{\hbar}(\boldsymbol{\sigma} \times \mathbf{p}) \cdot \mathbf{e_z} + \boldsymbol{m} \cdot \boldsymbol{\sigma} + \lambda k^3 \cos(3\theta)\, \sigma_z. \tag{3}$$

In the main text we provided the eigenstates and scatter function for an out-of-plane magnetic field, but here we give the general solution for arbitrary field directions. The dispersion is given by $E_{\pm} = \beta k^2 \pm p_\theta$, where $p_\theta = \sqrt{(\alpha k_x + m_x)^2 + (\alpha k_y - m_y)^2 + m_\theta^2}$. The $m_\theta$ term contains both the out-of-plane Zeeman term and the angle-dependent warping term, $m_\theta = m_z + \lambda k^3 \cos 3\theta$. The eigenfunctions are given by

$$\psi_{\pm} = \frac{1}{\sqrt{2p_\theta}} \begin{pmatrix} \frac{\alpha k i e^{-i\theta} + m_x - i m_y}{\sqrt{p_\theta - m_\theta}} \\ \pm\sqrt{p_\theta - m_\theta} \end{pmatrix}. \tag{4}$$

Scattering from $|\psi\rangle$ at zero angle to $|\psi'\rangle$ at angle $\theta$ is then given by $S_\pm = |\left\langle \psi'_\pm \,\middle|\, \psi_\pm \right\rangle|^2$, which provides us with the general solution,

$$S_\pm = \frac{1}{4}\frac{1}{p_\theta p_0}\frac{1}{(p_\theta - m_\theta)(p_0 - m_0)}\times \\ \Big[\left(\alpha^2 k^2 \cos\theta + m_x \alpha k \sin\theta - m_y \alpha k \cos\theta - m_y \alpha k + m_x^2 + m_y^2 + (p_\theta - m_\theta)(p_0 - m_0)\right)^2 \\ + \left(\alpha^2 k^2 \sin\theta - m_x \alpha k \cos\theta + m_x \alpha k - m_y \alpha k \sin\theta\right)^2\Big], \tag{5}$$

where $p_0 = p_\theta(\theta = 0)$ and $m_0 = m_\theta(\theta = 0)$. For relatively large warping and/or in-plane fields, it is straightforward to extend the expression to scattering from $\theta$ to $\theta'$ and to properly average scattering also over incoming angles.

In the limit when the magnetic field is out-of-plane ($m_x = m_y = 0$), our general solution can be written compactly as $S_\pm = \left[\frac{1}{2}\alpha^2 k^2 (1 + \cos\theta) + m_\theta^2\right] / (\alpha^2 k^2 + m_\theta^2)$, which is the expression given in the main text.

Now we focus on an in-plane field $\boldsymbol{B} = B_y \mathbf{e_y}$, perpendicular to the applied current ($\boldsymbol{I} = I_x \mathbf{e_x}$). The scatter factor is then given by

$$S_\pm = \frac{1}{4}\frac{1}{p_\theta p_0}\frac{1}{(p_\theta - m_\theta)(p_0 - m_0)}\times \\ \Big[\left(\alpha^2 k^2 \cos\theta - m_y \alpha k \cos\theta - m_y \alpha k + m_y^2 + (p_\theta - m_\theta)(p_0 - m_0)\right)^2 \\ + \left(\alpha^2 k^2 \sin\theta - m_y \alpha k \sin\theta\right)^2\Big], \tag{6}$$

which was used for the parallel field case of Fig. 3 in the main text.

It is also instructive to consider the parallel field case without warping. Then the scatter factor can be further simplified into

$$S_\pm = \frac{1}{2}\left[1 + \frac{\alpha^2 k^2 \cos\theta - m_y \alpha k\,(\cos\theta + 1) + m_y^2}{p_\theta p_0}\right]. \tag{7}$$

Note that this scattering factor reduces to $\frac{1}{2}(1 + \cos\theta)$ when $m_y \to 0$. Backscattering is forbidden in absence of a magnetic field, but applying an in-plane field changes this rule. In case of $\theta = \pi$ the scattering factor reduces to

$$S_\pm = \frac{1}{2}\left[1 + \frac{-\alpha^2 k^2 + m_y^2}{|\alpha^2 k^2 - m_y^2|}\right]. \tag{8}$$

If the magnetic field is sufficiently small ($m_y < \alpha k_F$), the scattering factor is equal to zero and backscattering is not allowed. However, upon increasing the magnetic field there is a sudden

jump in the scattering factor when the Zeeman energy equals to spin-orbit energy. The scattering factor is 1 if the Zeeman energy is larger than the spin-orbit energy. This sudden change in back-scattering contrasts the smooth behavior for an out-of-plane field. The intuitive picture is that an out-of-plane field gradually gives the spin orientation of the charge carriers an out-of-plane component. For the in-plane field some spins are already completely aligned with the magnetic field. Their backscattering companions are therefore initially pointing in the reverse field direction. The sudden jump in the scattering factor for $\theta = \pi$ occurs when the field gets large enough to flip those spins around to point towards the same orientation as the magnetic field. In this situation all spins have an overlap with the spins on the opposite of the Fermi circle. This change in the backscattering can also be recognized in the dispersion curve of Fig. 3a. If the crossing of the bands occur below the Fermi energy, the backscattering factor is equal to zero. Upon increasing the magnetic field, the crossing moves above the Fermi energy and the backscattering factor changes to 1.

### 4. Larger $E_{SO}$ in $Bi_2Te_3$ thin films

Thin films of $Bi_2Te_3$ are grown on $Al_2O_3$(0001) substrates using molecular beam epitaxy (MBE) by co-evaporating high purity Te (99.999%) and Bi (99.999%) in a Te rich environment. The base pressure of the MBE is lower than $5 \times 10^{-10}$ mbar, while the highest pressure recorded during growth is $4 \times 10^{-8}$ mbar. During deposition, the flux ratio Te/Bi is kept at about 10 and the growth rate at 4 Å/min. In order to avoid disordered interfacial layers at the interface between the film and the substrate, a two-step temperature growth scheme is used [3, 4]. This method results in atomically sharp interfaces. The first nucleation layer with a thickness of 10 nm is deposited at 190 °C, and then slowly annealed to the higher growth temperature of 230 °C in order to improve the crystalline quality. This annealed layer serves as a template for the subsequent epitaxial growth of the second layer (60 nm). After growth, the films are further annealed at 230 °C for 30 min to improve the film surface smoothness and quality, and subsequently cooled down to room temperature at a rate of 3 °C/min. This growth procedure yields high quality $Bi_2Te_3$ films with large terraces. Details on the growth procedure and systematic characterizations are presented in Ref. 5. The 70 nm film is structured into Hall bars (inset of Fig. S2) by means of optical lithography and Ar ion beam etching. The magnetoconductivity is shown in Fig. S2. Assuming the same band mass term of $\beta = 45$ eVÅ$^2$ as for the Hall bar in the main text, the Fermi energy is determined

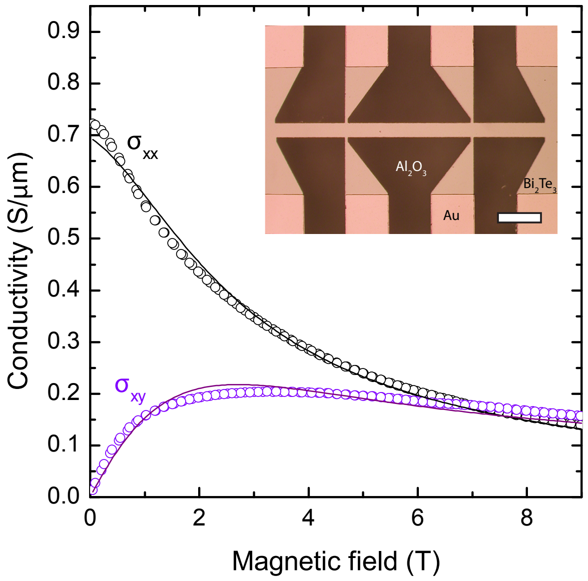


FIG. 2: **Figure S2 — Magnetoconductivity in $Bi_2Te_3$ thin film.** The Hall bar (see inset) was structured into a 70 nm thin film grown by molecular beam epitaxy on $Al_2O_3$. The scale bar indicates 150 μm. The longitudinal conductivity $\sigma_{xx}$ and transverse conductivity $\sigma_{xy}$ (circles) are obtained from the measured longitudinal and transverse resistivities. The magnetoconductance is fitted (solid lines) with the helical magnetoresistance model using similar parameters as for the flakes described in the main text.

from the Hall carrier density ($1/eR_H = 1.1 \times 10^{14}$ cm$^{-2}$) and calculated to be 42 meV. The best fit is found for a zero-field mobility of $\mu = 3250$ cm$^2$V$^{-1}$s$^{-1}$ and a Zeeman-to-spin-orbit ratio $\frac{g\mu_B}{\alpha k_F} = 0.11$ T$^{-1}$. For a $g$-factor of 12, the spin-orbit parameter would be $\alpha = 0.21$ eVÅ, slightly higher than obtained for the thicker flakes.

---


[1] M. Veldhorst, M. Snelder, M. Hoek, T. Gang, V. Guduru, X. Wang, U. Zeitler, W.G. van der Wiel, H. Hilgenkamp, A. Brinkman, Nature Mater. **11**, 417 (2012).

[2] M.s. Bahramy, P.D.C. King, A. de la Torre, J. Chang, M. Shi, L. Patthey, G. Balakrishnan, Ph. Hofmann, R. Arita, N. Nagaosa, F. Baumberger, Nature Comm. **3**, 1159 (2012).

[3] N. Bansal, Y.S. Kim, E. Edrey, M. Brahlek, Y. Horibe, K. Iida, M. Tanimura, G.-H. Li, T. Feng, H.-D. Lee, T. Gustafsson, E. Andrei, and S. Oh, Thin Solid Films **520**, 224 (2011).

[4] S. E. Harrison, S. Li , Y. Huo,B. Zhou, Y. L. Chen, and J. S. Harris, Appl. Phys. Lett. **102**,171906

(2013).

[5] P. Ngabonziza, R. Heimbuch, R.A. Klaassen, M. P. Stehno, M. Snelder, A. Solmaz, G. Koster, H. J. W. Zandvliet, and A. Brinkman, submitted for publication (2014).
